# Supplementary material for: Superconducting Phase of $\mathrm{Ti_xO_y}$ Thin Films Grown by Molecular Beam Epitaxy
Source: arXiv:2203.01405 source file (2022-12-01)
Supplement: Supplementary file 1 [file Supplemental_Materials.pdf]

# Supplemental Materials for "Superconducting Phase of $Ti_xO_y$ Thin Films Grown by Molecular Beam Epitaxy"

Yasemin Ozbek,[1] Cooper Brooks,[1] Xuanyi Zhang,[1] Athby Al-Tawhid,[1] Vladmir A. Stoica,[2] Zhan Zhang,[3] and Divine P. Kumah[1, *]

[1]Department of Physics, North Carolina State University, Raleigh, NC, 27695, USA

[2]Department of Materials Science and Engineering and Materials Research Institute,

Pennsylvania State University, University Park, PA 16802, USA

[3]Advanced Photon Source, Lemont, IL 76019, USA

**In-situ reflection high energy electron diffraction (RHEED)**

RHEED images taken after the growths of samples A,B,D,E and F are compared in Figure S1 along the $Al_2O_3$ $[10\bar{1}0]$ and $Al_2O_3$ $[11\bar{2}0]$ azimuths

| **Sample (Transport)** | **$Al_2O_3$ $[10\bar{1}0]$ direction** | **$Al_2O_3$ $[11\bar{2}0]$ direction** |
|---|---|---|
| A (I) | 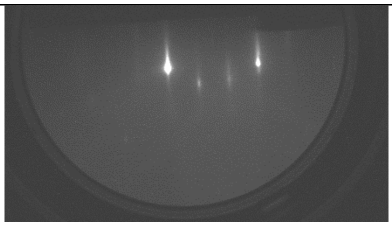 | 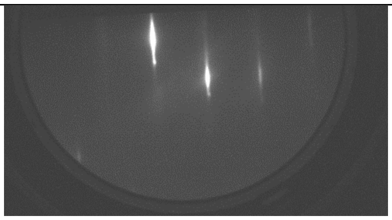 |
| B(M) | 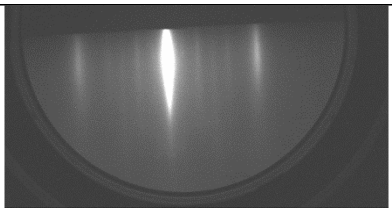 | 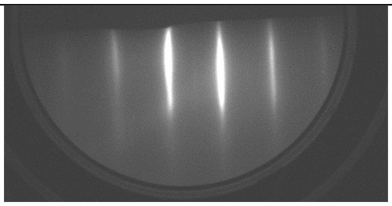 |
| D(M,SC) | 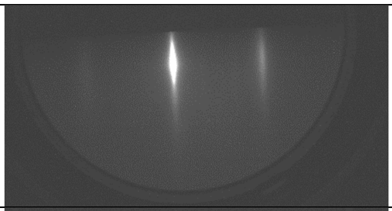 | 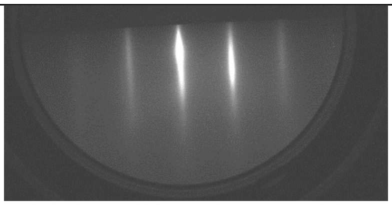 |
| E(I,SC) | 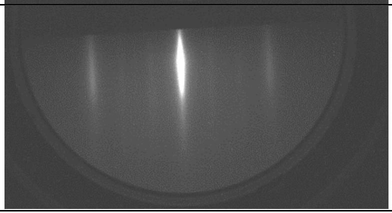 | 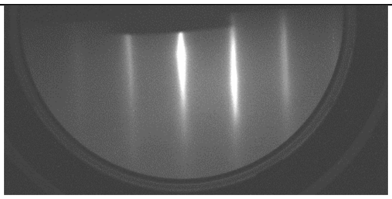 |
| F(Eutectic) | | 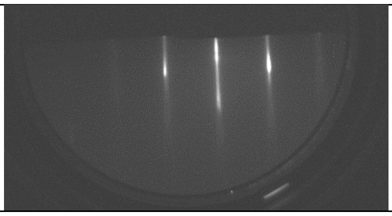 |
| | | |

*Figure S1: Reflection high energy electron diffraction images of $Ti_xO_y$ films grown by MBE*

**Atomic Force Microscopy.**

Figure S2 shows the atomic microscope image of an 85 nm $Ti_xO_y$ film grown on (0001)-oriented $\alpha - Al_2O_3$ . The step-like features observed for the film are identical to the as-prepared. The root-mean-square roughness is 0.7 nm.

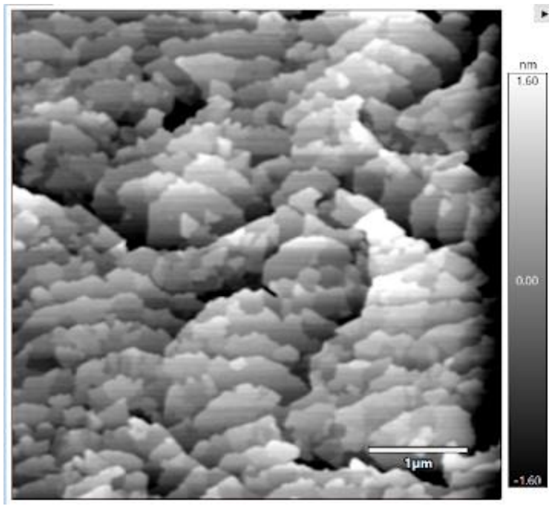


*Figure S2: Atomic force microscope image of 85 nm $Ti_xO_y$ film (Sample E) grown at $P_{ox}$=2x$10^{-7}$ Torr and $Ti_{rate}$=2.4x$10^{13}$ atoms/$cm^2$s*

**Optical Images of $Ti_xO_y$ films**

A comparison of optical images of the eutectic (sample F), metallic (Sample B) and superconducting (Sample E) is shown in Figure S3.

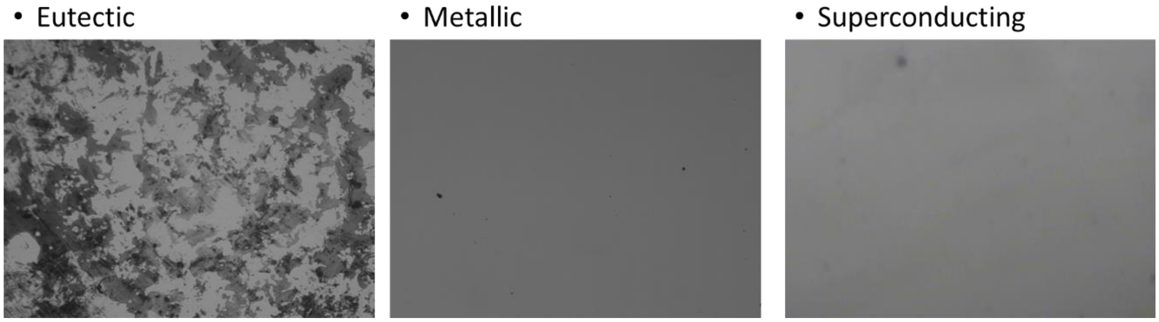


*Figure S3: Optical images of eutectic, metallic and superconducting $T_{ix}O_y$ films grown by molecular beam epitaxy on (0001)-$Al_2O_3$.*
